# Supplementary material for: Explainable Product Classification for Customs
Source: arXiv:2311.10922 source file (2023-11-18)
Supplement: Supplementary file 1 [file 9_supplementary.tex]

\section{Dataset}
\subsection{Dataset Example}

\begin{figure}[t]
\centerline{
      \includegraphics[width=\linewidth]{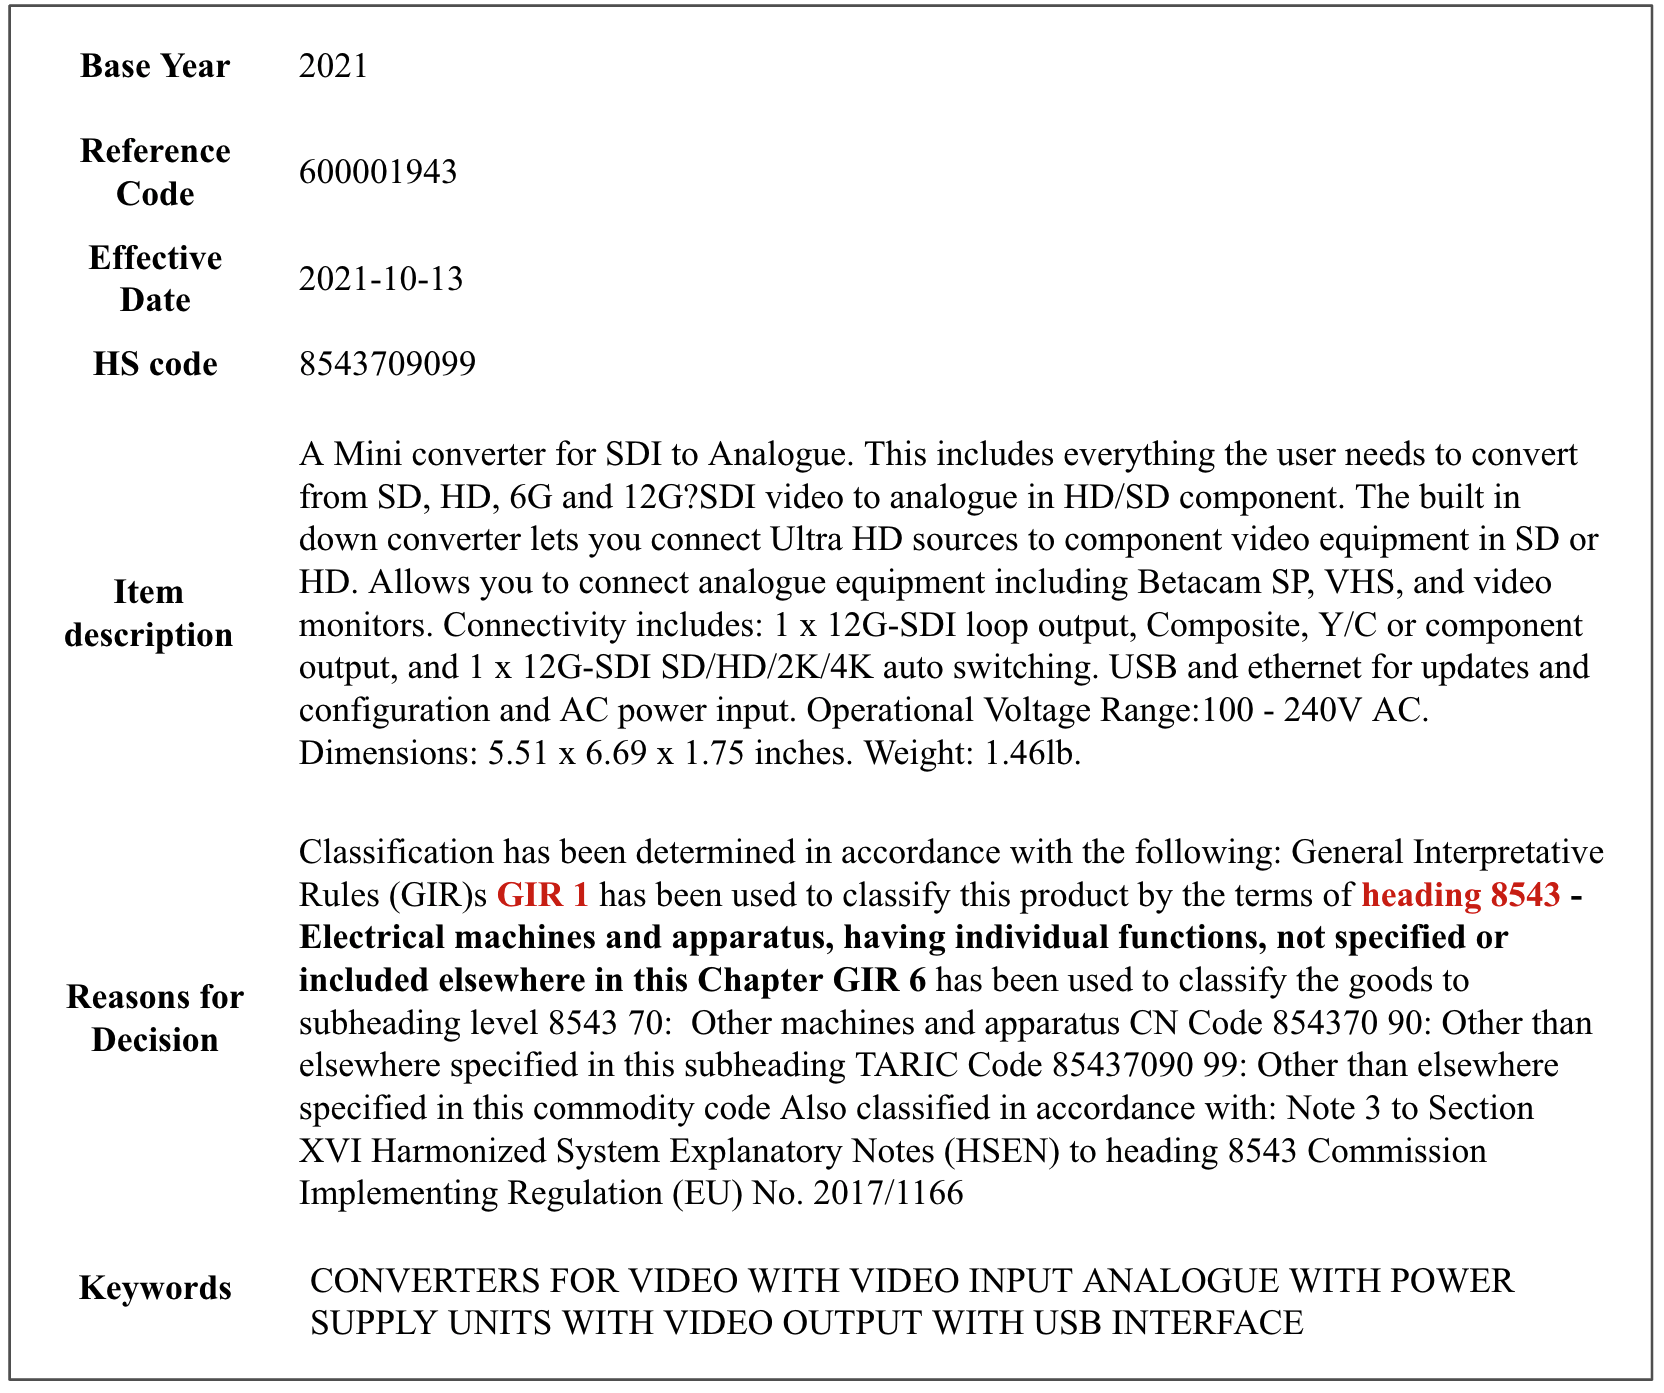}}
      \caption{Illustration of a decision case including item description and corresponding HS code. Explanations of item's Chapter, Heading and Subheading are also given.
    %   \mc{Make it shorter by half?}
      } 
\label{fig:model}
\end{figure}

\begin{figure}[t]
\centerline{
      \includegraphics[width=\linewidth]{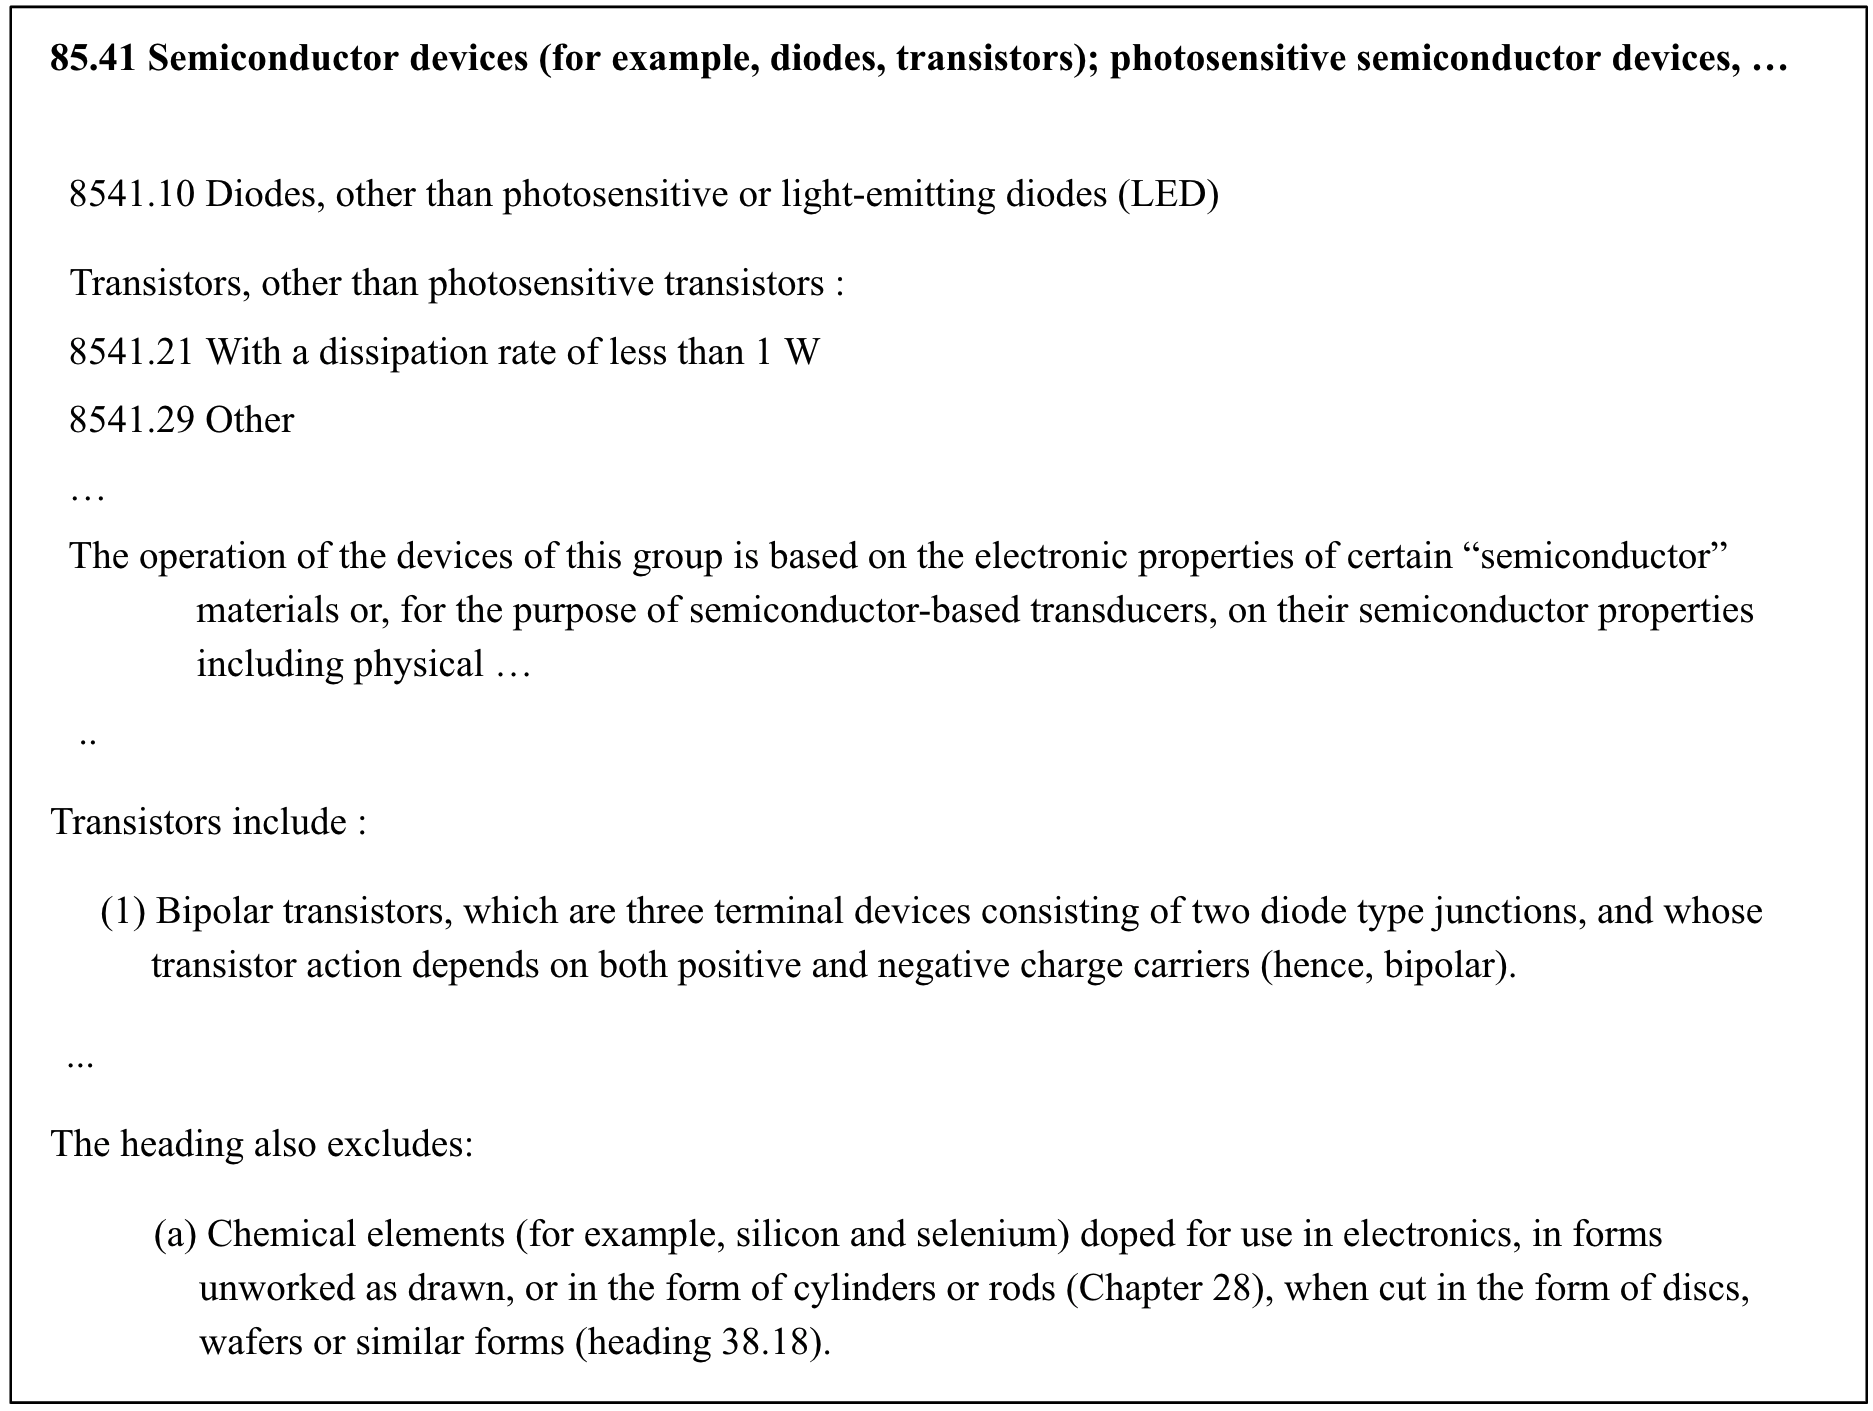}}
      \caption{An example of the heading-level explanation in HS manual. Manual provides characteristics and standards of each heading (8541 here) in detail, and it includes one-liner description of every subheadings.
    %   \mc{Make it shorter by half? Maybe combine with Fig 1?}
      } 
\label{fig:HS_manual}
\end{figure}

\section{Case study}
We now describe how the supporting model predicted with two concrete examples-- each being a correct prediction and a wrong prediction. The difference between the two cases happens since they are concentrated on different terms. The mistake usually occurs when another HS code shares a similar concept. The suggested model might miss the HS answer in the predicted candidate set, but it can still provide important sentences from the relevant HS manual.

\subsection{Case1 : Correct Prediction}

\subsubsection{Given item description. \quad}
-A device that generates compressed air for brake operation of commercial vehicles such as electric buses and hydrogen trucks.
-Specification: Rated power consumption of 3kW, maximum power consumption of 10kW, the pressure of 10bar.
-Operation Principle: The crankshaft rotates with the rotational force transmitted through the motor. The connecting rod and piston loaded on the shaft convert the rotational force into a straight reciprocating motion. Air is introduced, compressed, and discharged through a straight round trip.
-Equipped vehicles: Electric buses, hydrogen trucks, etc.

\subsubsection{Answer HS code. \quad}
\begin{itemize}
    \item \textbf{8414.80} - Air or vacuum pumps, air or other gas compressors and fans; ventilating or recycling hoods incorporating a fan, whether or not fitted with filters. : Other
\end{itemize}

\subsubsection{Predicted HS code. \quad}
\begin{itemize}
    \item \textbf{8414.80} - Air or vacuum pumps, air or other gas compressors and fans; ventilating or recycling hoods incorporating a fan, whether or not fitted with filters. : Other
    \item \textbf{8414.59} - Air or vacuum pumps, air or other gas compressors and fans; ventilating or recycling hoods incorporating a fan, whether or not fitted with filters. : Fans : Other
    \item \textbf{8428.20} - Other lifting, handling, loading or unloading machinery (for example, lifts, escalators, conveyors, teleferics). : Pneumatic elevators and conveyors

\end{itemize}

\subsubsection{Retrieved sentences. \quad}
\begin{itemize}
    \item 84.14 - Air or vacuum pumps, air or other gas compressors and fans; ventilating or recycling hoods incorporating a fan, whether or not fitted with filters.
    \item Those of the first kind may act as air extractors or as blowers (e.g., industrial blowers used in wind tunnels). 
    \item This heading covers machines and appliances, hand-operated or power driven, for the compression of air or other gases, or for creating a vacuum, and also machines for circulating air or other gases.
    \item In general, air pumps, vacuum pumps and compressors function on the same principles as and are broadly of similar construction to the liquid pumps (piston, rotary, centrifugal or ejector pumps) described under the preceding heading.

\end{itemize}

\subsubsection{Case analysis. \quad}
The given item is an air pump device for commercial vehicles, so it should be classified into \textit{8414.80}. In this case, our model chooses four sentences from \textit{8414} HS manual. It includes a description of the heading, an explanation of items that belonged here, and a description of the air pump. These are helpful information for classification, as users can learn candidate HS code characteristics and understand important terminologies here.  

\subsection{Case2 : Tricky Case}

\subsubsection{Given item description. \quad} 
Item Overview of items
- It is a 12-inch monitor that is directly connected to an automatic data processing machine in industrial automation facilities and outputs various operation buttons and machine operation status on the TFT-LCD (1,280*800 pixels) screen, and has an integrated touch screen (analog resistance film) that functions as an operation button.
- It consists of a power supply (Power), an operation unit (touch screen), and a display unit (TFT-LCD*), and operates with a Windows CE 6.0 system (embedded O/S in an automatic data processing device).
* Display data conversion and scaling (adjustment of magnification, rotation, etc.) functions are possible.
Near Degree of association with peripherals ( This Automatic data processing machine directly connected to this building)
- It is a gateway processor that interconnects various devices in the industrial field and central computers in office space on the network, and is a controller of Human Machine Interface (HMI) used for PLC purposes as an automatic control controller when mounted on individual machines.
- Main specification.
CPU : Intel ATOM E660 or E680, 1.30GHz, 32-bit Operating System
Main Memory: Micron Technology MT47H256M8EB-25EIT:C(256MB×8)
Secondary Storage : SD CARD 4GB & CFast CARD 16GB
Port: 3 USB 2.0 (Type A), 1 USB 2.0 (mini B), 2 Ethernet, 2 COMs (connected with various controllers), DVI-D output, extended unit (industrial network connection)

\subsubsection{Answer HS code. \quad}
\begin{itemize}
    \item \textbf{8528.52} - Monitors and projectors, not incorporating television reception apparatus; reception apparatus for television, whether or not incorporating radio-broadcast receivers or sound or video recording or reproducing apparatus. : Capable of directly connecting to and designed for use with an automatic data processing machine of heading 8471
\end{itemize}

\subsubsection{Predicted HS code. \quad}
\begin{itemize}
    \item \textbf{8471.41} - Automatic data processing machines and units thereof; magnetic or optical readers, machines for transcribing data onto data media in coded form and machines for processing such data, not elsewhere specified or included : Comprising in the same housing at least a central processing unit and an input and output unit, whether or not combined 
    \item \textbf{8472.90} - Other office machines : Other 
    \item \textbf{8471.49} - Automatic data processing machines and units thereof; magnetic or optical readers, machines for transcribing data onto data media in coded form and machines for processing such data, not elsewhere specified or included : Other, presented in the form of systems
\end{itemize}

\subsubsection{Retrieved sentences. \quad}

\begin{itemize}
    \item 84.71 Automatic data processing machines and units thereof; magnetic or optical readers, machines for transcribing data onto data media in coded form and machines for processing such data, not elsewhere specified or included.
    \item (i) It is of a kind solely or principally used in an automatic data processing system;
    \item X-Y co-ordinate input devices, which are units for inputting position data into automatic data processing machines. 
    \item (2) An input unit which receives input data and converts them into signals which can be processed by the machine.
\end{itemize}

\subsubsection{Case analysis. \quad}
The given item is a monitor connected to an automatic data processing machine. Therefore, it should be classified into \texit{8528.52}, which is a code for monitors and projectors. Our algorithm suggested different HS since it concentrated on term \textit{automatic data processing machines}, not the \textit{monitor}. Accordingly, the model provided two candidates from heading \textit{8471}, which is for \textit{automatic data processing machines and units thereof}. This happens since heading \textit{8471} and subheading \texit{8528.52} are closely related. From Customs Law Information Portal (CLIP), four cases were classified into \texit{8528.52} by the HS Committee. 

In all of these four cases, experts quoted sentences from \textit{8471} HS manual in reasons for the decision. Experts decide whether the item belongs to \textit{8471} or not, referring to these sentences from the HS manual. Sentences retrieved by our algorithm are from \textit{8471} HS manual, and these sentences explain what an automatic data processing machine and its unit are which examples it includes. Our model made a mistake in the final decision but provided essential information (sentences from \textit{8471} HS manual) for a classification task. Here, we could know that even if the model missed the answer HS, it could still do its role as a supporting model.
